# Supplementary material for: Gaze-LLE: Gaze Target Estimation via Large-Scale Learned Encoders
Source: arXiv:2412.09586 source file (2025-06-04)

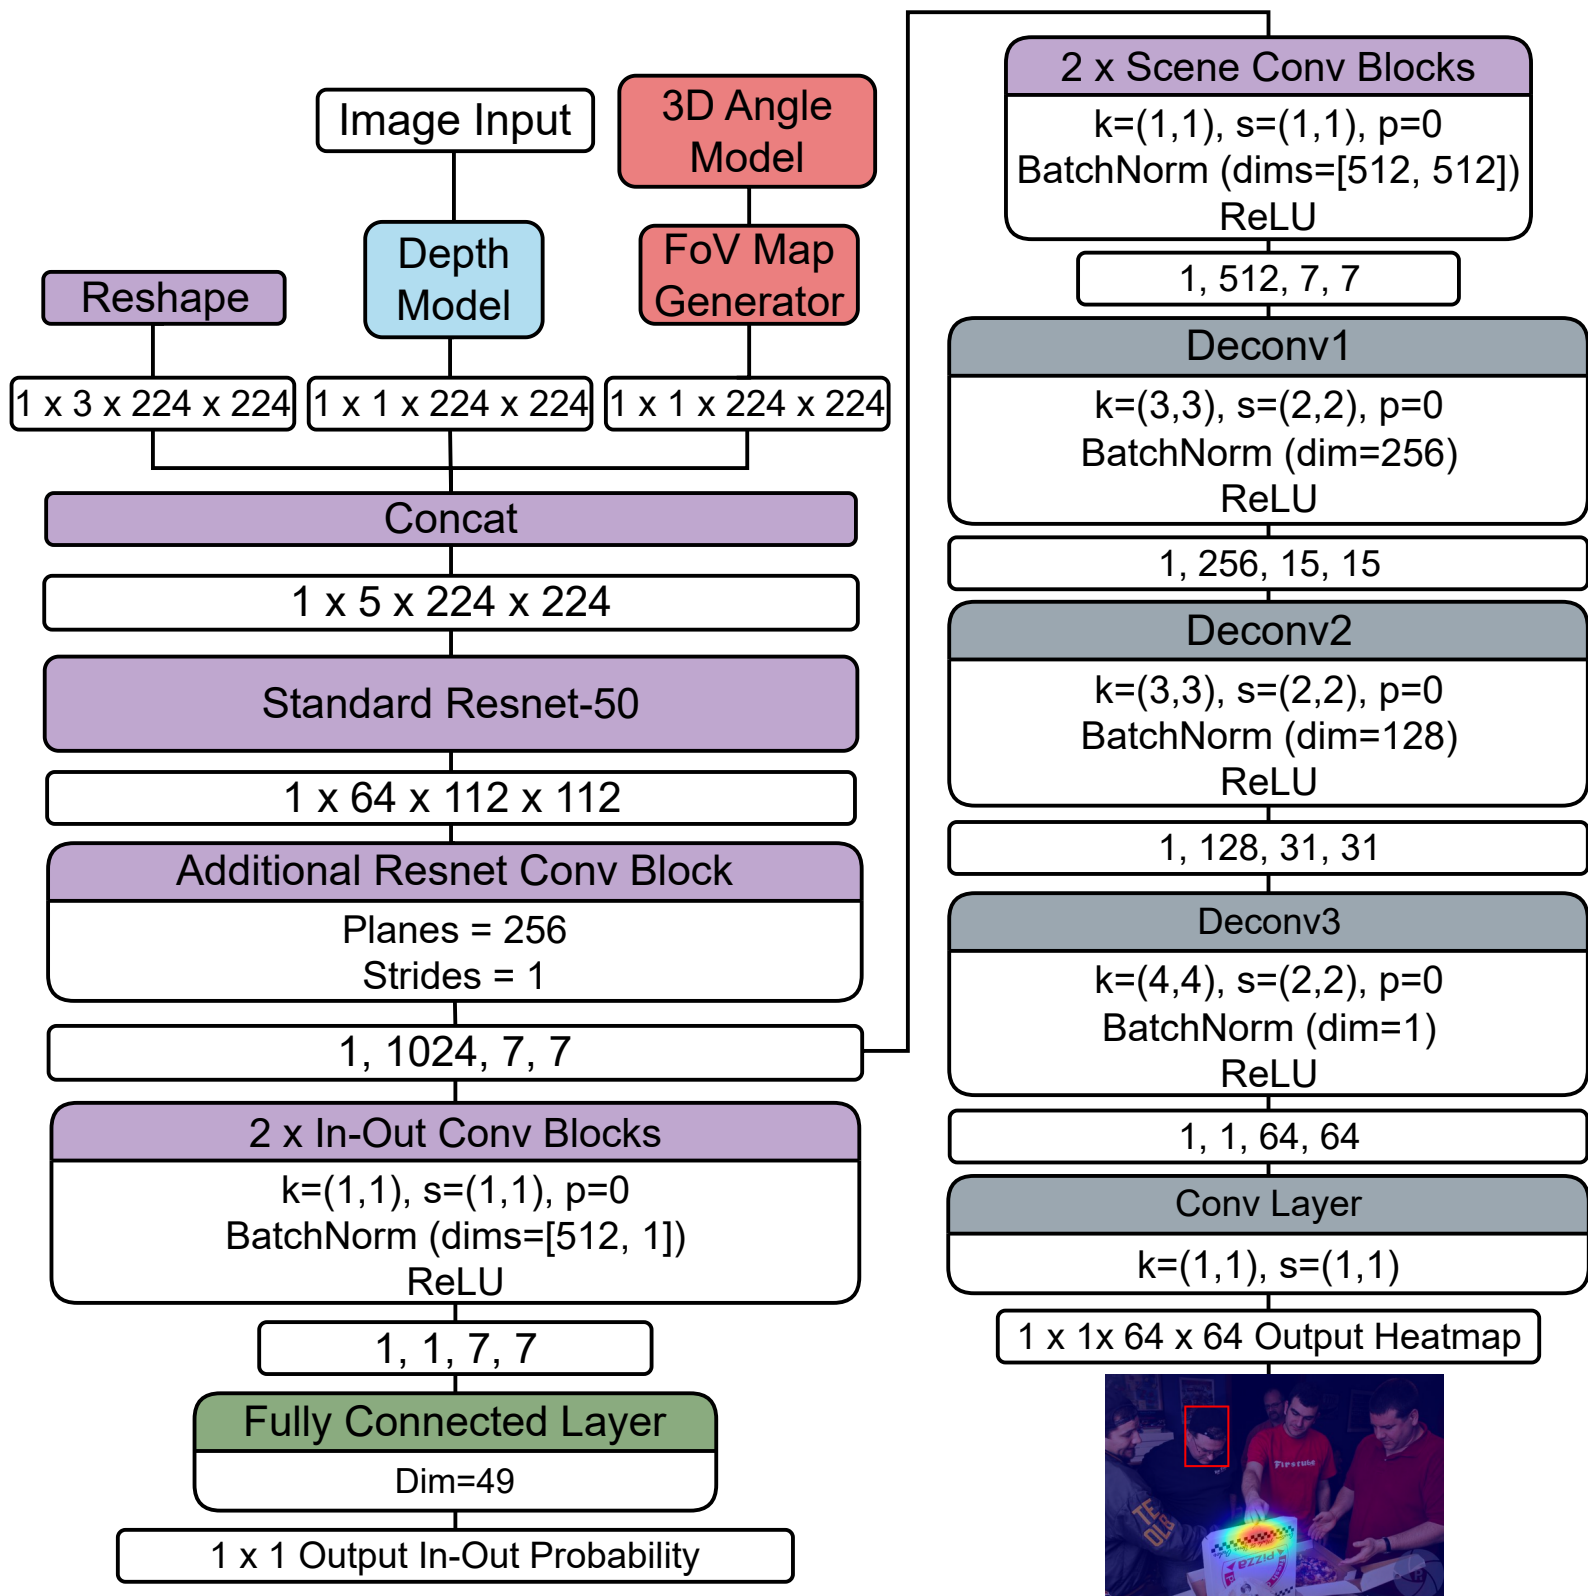

## FoV Map Generator

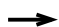

## FoV Map Generator

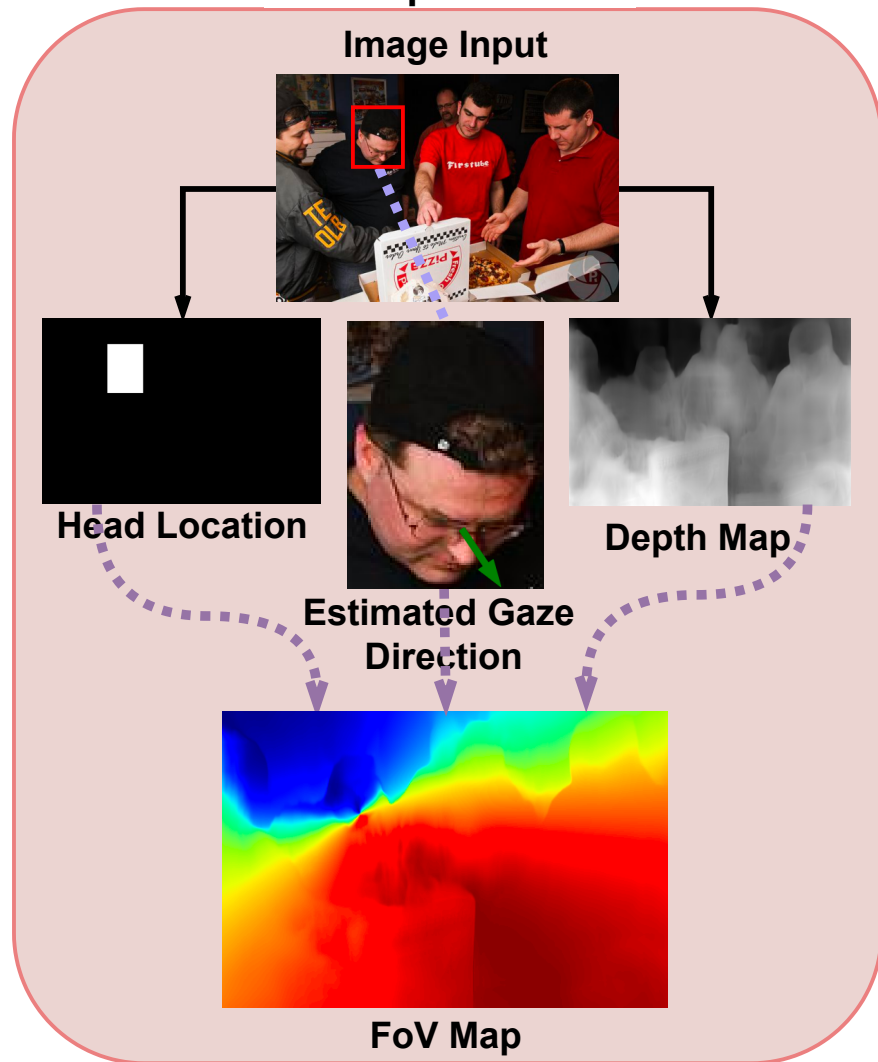

## FoV Map Generator

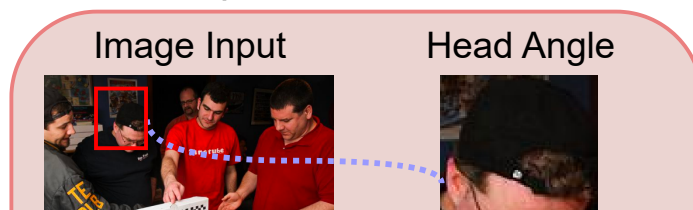

Supplement: Supplementary file 1 [file horanyiModel2.pdf]
